# Supplementary material for: Uncertainties of Latent Representations in Computer Vision
Source: arXiv:2408.14281 source file (2024-08-26)
Supplement: Supplementary file 1 [file appendix.tex]

\section{Method}
